# Supplementary material for: Variable and orbital-dependent spin-orbit field orientations in a InSb double quantum dot characterized via dispersive gate sensing
Source: arXiv:2203.06047 source file (2022-04-12)
Supplement: Supplementary file 1 [file Suppl.pdf]

# SUPPLEMENTARY MATERIAL: Variable and orbital-dependent spin-orbit field orientations in a InSb double quantum dot characterized via dispersive gate sensing

Lin Han[1,*] Michael Chan[1], Damaz de Jong[1], Christian Prosko[1], Ghada Badawy[2], Sasa Gazibegovic[2], Erik P.A.M. Bakkers[2], Leo P. Kouwenhoven[1], Filip K. Malinowski[1,†] and Wolfgang Pfaff[3]

[1] QuTech and Kavli Institute of Nanoscience, Delft University of Technology, 2600 GA Delft, The Netherlands

[2] Department of Applied Physics, Eindhoven University of Technology, MB Eindhoven, 5600, The Netherlands

[3] Department of Physics and Frederick Seitz Materials Research Laboratory, University of Illinois at Urbana-Champaign, Urbana, IL 61801, USA

## A. EXTRACTION OF $C_q$

In this section, we describe how quantum capacitance $C_q$ in this letter is acquired and analyzed. The $C_q$ is extracted via calculating the changes of the capacitive load on the resonator from its bare value, as it results in a resonance frequency shift $\Delta f$ that is directly obtainable from measurements [1]:

$$C_q = C - C_{cb} = \frac{1}{(2\pi)^2(f_{cb}+\Delta f)^2 L} - \frac{1}{(2\pi)^2 f_{cb}^2 L}. \quad (1)$$

Here, $C$ is the effective capacitance being measured, $L$ is fixed to be 730 nH. $C_{cb}$ and $f_{cb}$ are the capacitance and resonance frequency at Coulomb blockade, respectively. According to this equation, the value of $f_{cb}$ and $\Delta f$ are required to know to get $C_q$.

The measurement of $C_q$ at given gate settings under a certain external magnetic field consists of two steps. In the first step, we fix the gate settings near the interdot charge transition (ICT) that we aim to study (similar to Fig. 1(b)), and measure the frequency dependence of the reflection coefficient $S_{11}$ around the resonance frequency $f_0$ (e.g. Fig. S1(a)). Consider the hanger geometry of the coupled resonator, we fit the measured $S_{11}$ with the resonator model inspired by Khalil et al. [2], where they derive the transmission coefficient $S_{21}$ of the hanger resonator. At probing frequency $f_p$, the measured $S_{11}$ differs from $S_{21}$ by a factor of 2 to convert from hanger geometry to reflection:

$$S_{11} = 1 - \frac{2e^{i\phi}\frac{Q}{Q_e}}{1+2iQ\frac{f_p - f_0}{f_0}}. \quad (2)$$

Here, $Q = 1/(1/Q_i + 1/Q_e)$ is the total quality factor, with $Q_{i(e)}$ being the internal (external) quality factor [3, 4]. The asymmetry of reflection is captured by the phenomenological phase term $e^{i\phi}$, while is not originated from the impedance mismatch as in Ref. [2]. Therefore, we get the value of $f_0$ for that particular gate setting, and the corresponding parameters of the resonator, including $Q_i$, $Q_e$, and phase factor $\phi$. With this approach, the values of quality factors are not accurately defined, but the influence on analysis is negligible when they are fixed in our case. Fig. S1(a,b) show an example of the fitting results comparing to the raw data in both amplitude response and in I-Q plane. In the second step, we set the probing frequency to $f_p$, and measure the charge stability diagram (CSD) that completely encompasses the target ICT (see Fig. S1(c)).

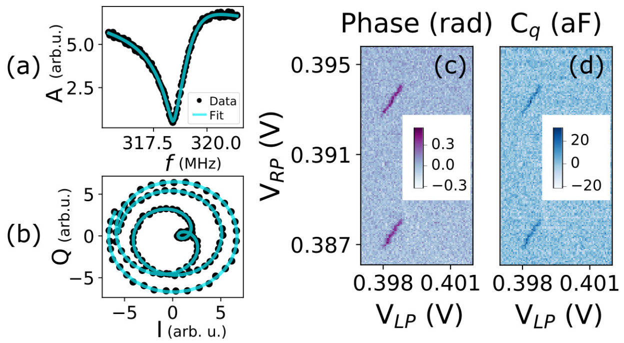


Figure S1. (a) The magnitude of the reflection signal as a function of probing frequency, as an example of the reference data. The black dots represents the raw data, while the blue curve shows the fitting result. (b) Parametric plot of the resonator reflection measurement in I-Q plane, and the corresponding fit result. (c) The reflected phase signal of the entire charge stability diagram. (d) The corresponding color maps of $C_q$ values.

We now assume all resonator parameters are fixed within the gate voltage space of that CSD, except for $C_q$ that changes the resonance frequency by $\Delta f$. As the probing frequency $f_p$ is known, we calculate all the corresponding $S_{11}$ with different resonance frequency $f_0$, according to the resonator model in Eq. (2) with those fitted resonator parameters. Then, for each pixel $i$ in the CSD (eg. in Fig. S1(c)), we extract the value of $f_0^i$ with the measured $S_{11}^i$. The value of $f_{cb}$ is defined as a mean value of the resonance frequency $f_0^i$ away from any ICT. In this case, the resonance frequency shift $\Delta f^i$ is measured relative to $f_{cb}$. Finally, with Eq. (1), the values of $C_q^i$ in the scanned gate voltage space are extracted, as shown in Fig. S1(d)).

## B. MODELING THE DQD

In order to describe the effects observed in the DQD, we construct an effective Hamiltonian $\hat{H}_{tot}$ for the system in the Hund-Mulliken approximation using the sec-

ond quantization notation [5, 6]. Only one orbital per dot, which can be doubly occupied by electrons, is considered in this approximation. In our model, $\hat{H}_{tot}$ consists of an electrostatic term $\hat{H}_e$, a magnetic Zeeman term $\hat{H}_m$ and a spin-orbit interaction (SOI) term $\hat{H}_{so}$:

$$\hat{H}_{tot} = \hat{H}_e + \hat{H}_m + \hat{H}_{so}. \tag{3}$$

Formally, SOI mixes the orbital and spin part of the electron wave function, and results in Kramers doublets. They are referred to as the conventional spin doublets: an external magnetic field $\mathbf{B}$ induces a Zeeman splitting between the spin doublets. The SOI itself is modeled as an effective electron momentum dependent magnetic field $\mathbf{B}_{so}$, around which the spin of the tunneling electron precesses[7]. We use a phenomenological interaction Hamiltonian of the form of

$$\hat{H}_{so} = \mathbf{B}_{so}(\hat{p}_x, \hat{p}_y, \hat{p}_z) \cdot \hat{\sigma}, \tag{4}$$

where $\hat{p}_i$ is the momentum operator in the three Cartesian directions $(i = x, y, z)$, and $\hat{\sigma}$ is the Pauli (spin-1/2) operators. In particular, we define the spin basis of the electron such that the spin quantization axis (the projection of the spin on z-axis) aligns with $\mathbf{B}$. The angle $\eta$ is defined as the angle associated with the inner product of $\mathbf{B}$, thus $\mathbf{B}_{so}$ allowing us to decompose $\mathbf{B}_{so}$ into a parallel and perpendicular component with respect to the spin quantization axis. For simplicity, we choose the projection of the spin on the y-axis align with the component of $\mathbf{B}_{so}$ that is perpendicular to $\mathbf{B}$. The SOI Hamiltonian is therefore given as

$$\begin{aligned}\hat{H}_{so} = it_p \sum_{\alpha,\beta=\{\uparrow,\downarrow\}} \Big( &\cos(\eta)\, \hat{c}^\dagger_{L,\alpha} \sigma_z^{\alpha\beta} \hat{c}_{R,\beta} \\ &+ \sin(\eta)\, \hat{c}^\dagger_{L,\alpha} \sigma_y^{\alpha\beta} \hat{c}_{R,\beta} - \, h.c.\Big),\end{aligned} \tag{5}$$

where $t_p$ is the spin precessing tunnel coupling due to SOI, while $\sigma_{y(z)}$ is the spin $\frac{1}{2}$ Pauli y-(z-) matrices. $\hat{c}^\dagger_{i,\sigma}$ and $\hat{n}_{i,\sigma}$ are the fermionic creation and number operator for the electrons in dot $i$ with spin $\sigma$.

Together with

$$\begin{aligned}\hat{H}_e = \frac{\epsilon}{2} &\sum_{\sigma,\sigma'=\{\uparrow,\downarrow\}} \left(\hat{n}_{L,\sigma} - \hat{n}_{R,\sigma'}\right) \\ &+ t \sum_{\sigma} \left(\hat{c}^\dagger_{L,\sigma} \hat{c}_{R,\sigma} + h.c.\right) \\ &+ \sum_{i=\{L,R\}} \left(U_i \hat{n}_{i,\uparrow} \hat{n}_{i,\downarrow}\right),\end{aligned} \tag{6}$$

and

$$\begin{aligned}\hat{H}_m = -\frac{\mu_B B}{2} &\big(g_L(\hat{n}_{L,\uparrow} - \hat{n}_{L,\downarrow}) \\ &+ g_R(\hat{n}_{R,\uparrow} - \hat{n}_{R,\downarrow})\big),\end{aligned} \tag{7}$$

we obtain the full Hamiltonian of the DQD system. Here, $\epsilon$ is the detuning, $t$ is the spin conserving tunnel coupling, and $U_{L(R)}$ is the Coulomb repulsion induced energy cost for placing two electrons on the same left(right) dot. Moreover, $\mu_B$ denotes the Bohr magneton, $B$ the external field magnitude and $g_{L(R)}$ the Landé g factor of the left(right) dot.

For ICTs between the $|(2,0)\rangle$ and $|(1,1)\rangle$ charge states, the following even parity states are of relevance:

$$\begin{aligned}|(2,0)S\rangle &= \hat{c}^\dagger_{L,\uparrow} \hat{c}^\dagger_{L,\downarrow} |0\rangle \\ |(1,1)S\rangle &= \frac{1}{\sqrt{2}} \left(\hat{c}^\dagger_{L,\uparrow} \hat{c}^\dagger_{R,\downarrow} - \hat{c}^\dagger_{L,\downarrow} \hat{c}^\dagger_{R,\uparrow}\right) |0\rangle \\ |T_+\rangle &= \hat{c}^\dagger_{L,\uparrow} \hat{c}^\dagger_{R,\uparrow} |0\rangle \\ |T_0\rangle &= \frac{1}{\sqrt{2}} \left(\hat{c}^\dagger_{L,\uparrow} \hat{c}^\dagger_{R,\downarrow} + \hat{c}^\dagger_{L,\downarrow} \hat{c}^\dagger_{R,\uparrow}\right) |0\rangle \\ |T_-\rangle &= \hat{c}^\dagger_{L,\downarrow} \hat{c}^\dagger_{R,\downarrow} |0\rangle,\end{aligned} \tag{8}$$

with $|0\rangle$ being a vacuum state.

For $B = 0$, we can project $\hat{H}_{tot}$ onto this basis and analytically diagonalize the Hamiltonian to find the ground state energy

$$E_g = \frac{1}{2}\left((U_L + \epsilon) - \sqrt{(U_L + \epsilon)^2 + 8(t^2 + t_p^2)}\right). \tag{9}$$

Note that $U_L$ offsets (the onset of) the avoided crossing along the detuning axis only and can be set to zero by redefining the detuning axis. The $C_q$ value can then be calculated as the curvature of the ground state energy $-\left(e\alpha'\right)^2 \frac{\partial^2 E_g}{\partial \epsilon^2}$, for which we find ($\alpha'$ is the effective lever arm accounted for cross coupling) [8–10]

$$C_{q,B=0} = \frac{(e\alpha')^2}{2} \frac{8t_{tot}^2}{\left(\epsilon^2 + 8t_{tot}^2\right)^{\frac{3}{2}}}, \tag{10}$$

where $e$ is the elementary charge. In addition, we define $t_{tot} = \sqrt{t^2 + t_p^2}$ as the total tunnel coupling set by the barrier gates.

Another special limit is when $\mathbf{B} \perp \mathbf{B}_{so}$, where $\eta = \pi/2$. According to $\hat{H}_{so}$, the spin flipping due to SOI during tunneling is strongest. When the Zeeman energy $E_z$ is the second largest energy scale ($E_z >> t_{tot}$), we expect that the ground state is solely contributed to by the states $|(2,0)S\rangle$ and $|T_+\rangle$ that are coupled by SOI through the tunneling element $t_p$. In this case, the ground and first excited state are analytically approximated by projecting $\hat{H}_{tot}$ onto the aforementioned two states. The ground state energy and $C_q$ are found as

$$\begin{aligned}E_g &= \frac{1}{2}\Big[U_L + \epsilon - \frac{\mu_B B}{2}(g_L + g_R) \\ &\quad - \sqrt{\left(U_L + \epsilon + \frac{\mu_B B}{2}(g_L + g_R)\right)^2 + 4t_p^2}\Big]; \\ C_{q,B\perp B_{so}} &= \frac{2(e\alpha')^2 t_p^2}{\left[(U_L + \epsilon + \frac{\mu_B B(g_L + g_R))^2}{2} + 4t_p^2\right]^{\frac{3}{2}}}.\end{aligned} \tag{11}$$

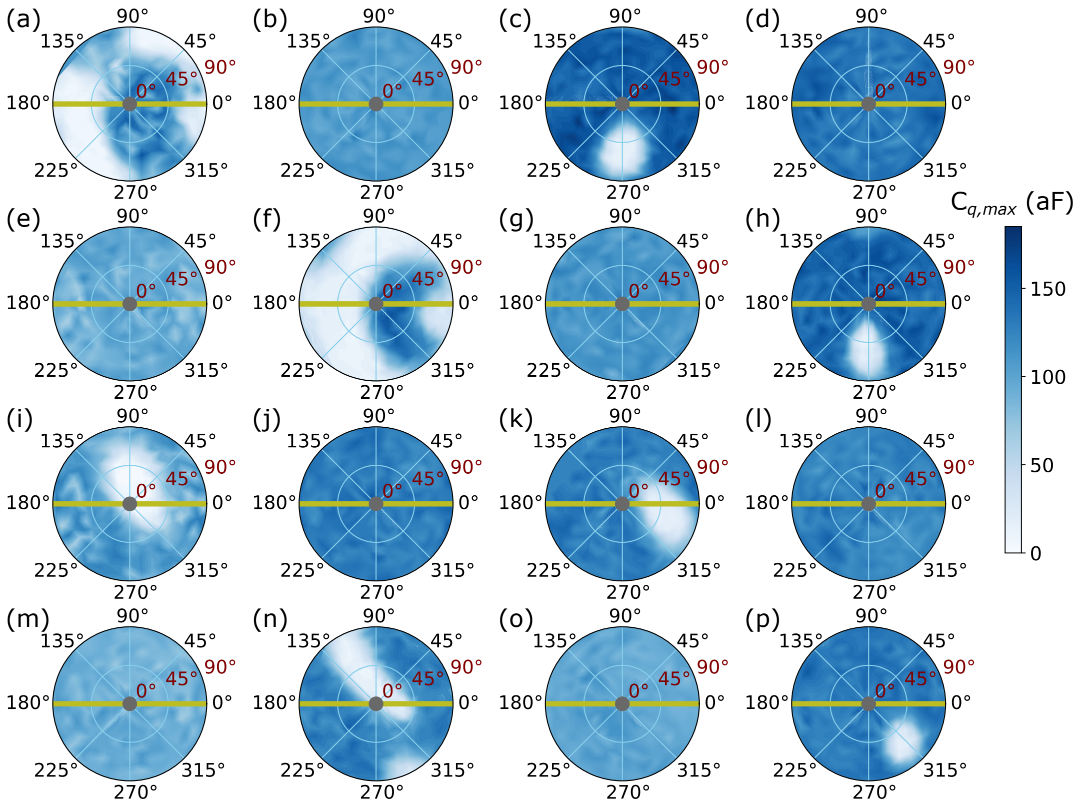


Figure S2. Magnetic field angle maps of $C_{q,max}$ for a set of 16 adjacent ICTs. The positions of those maps in the plot correspond to the relative positions of the ICTs in a CSD, just like in Fig. 1(b). We identify the transitions corresponding to panels (b,d,e,g,j,l,m,o) are of total odd occupancy of the double quantum dot. Panels (i) and (n) correspond to Fig. 4(b) and (c), while (c) and (h) corresponds to Fig. 4(d) and (e). Irregular regions of $C_{q,max}$ suppression in (a,f,n) are discussed in terms of topologically protected Weyl points in the main text. We also suspect that the g-factors of the ICTs in (a,f) are larger than other ICTs, thus sweeping with smaller external field is preferred.

For the more general case, we employ numerical simulations to compute $C_q$. We project the five spin basis states (in Eq. (8)) onto $\hat{H}_{tot}$ and numerically diagonalize it to find the eigenenergies $E_n$ and states $\Psi_n$. In the limit of relaxation rates being slower than the probing frequency, $C_q$ is calculated as the curvature of the energy bands, or equivalently through $\left(e\alpha'\right)^2 \frac{d\langle n_L\rangle}{d\epsilon}$ [11]. In thermal equilibrium, $C_q$ can be expressed as

$$C_q = \left(e\alpha'\right)^2 \sum_n \frac{e^{-\frac{E_n(\epsilon)}{k_B T}}}{\mathcal{Z}} \left(\frac{d\left\langle \Psi_n|\hat{n}_L|\Psi_n\right\rangle(\epsilon)}{d\epsilon}\right), \quad (12)$$

where $k_B$ is the Boltzmann constant, $T$ is the electronic temperature, and $\mathcal{Z} = \text{Tr}\left(e^{-\frac{\hat{H}_{tot}}{k_B T}}\right)$ is the partition function. $\frac{d\langle n|\hat{n}_R|n\rangle(\epsilon)}{d\epsilon}$ itself is numerically computed using the central difference method.

### C. $\mathbf{B}_{SO}$ field orientation of adjacent ICTs

In the gate voltage space along $V_{LP}$ and $V_{RP}$, we study 4-by-4 array of neighboring ICTs. With the magnitude of external magnetic field fixed at 50 mT, we measure the magnetic field angle map of $C_{q,max}$ for all those 16 ICTs. Fig. S2 presents color maps of the extracted $C_{q,max}$ for those ICTs, in a polar-type projection (similar in Fig. 2(d) with $0° \leq \theta \leq 90°$). The maps are arranged according to their relative position in gate voltage space. Since the inversion symmetry of $\pm\mathbf{B}_{SO}$ is already demonstrated in Fig. 2, we measure the $C_{q,max}$ values only for one hemisphere.

Fig. S2(c,h,i,n) correspond to Fig. 4(b,c,d,e), respectively. It is clearly shown with Fig. S2(b,d,e,g,j,l,m,o) that for ICTs with odd total parity, $C_{q,max}$ values are independent of the orientation of the external magnetic field. When an ICT is for even total parity, the $\mathbf{B}_{SO}$ orientation can be identified from the suppression of $C_{q,max}$. In Fig. S2(a,f,n), there is possibility that more than 2 Weyl points exist [12]. The $C_{q,max}$ suppression regions in Fig. S2(a,f) are too large to fit $\mathbf{B}_{SO}$ orientations meaningfully, which may be due to a small level spacing to the first excited state.

## AUTHOR CONTRIBUTION

WP and FKM envisioned the experiment. LH fabricated the nanowire device. LH, FKM, MC performed the experiments and the data analysis. MC, FKM implemented the simulation model. GB, SG and EPAMB grew the InSb nanowire. LH wrote the manuscript with input from FKM, MC, WP, DdJ, CP, LK.

* L.Han-2@tudelft.nl
† F.K.Malinowski@tudelft.nl

[1] D. De Jong, J. Van Veen, L. Binci, A. Singh, P. Krogstrup, L. P. Kouwenhoven, W. Pfaff, and J. D. Watson, Physical Review Applied **11**, 044061 (2019).
[2] M. Khalil, M. Stoutimore, F. Wellstood, and K. Osborn, Journal of Applied Physics **111**, 054510 (2012).
[3] J. Van Veen, D. De Jong, L. Han, C. Prosko, P. Krogstrup, J. D. Watson, L. P. Kouwenhoven, and W. Pfaff, Physical Review B **100**, 174508 (2019).
[4] F. K. Malinowski, L. Han, D. de Jong, J.-Y. Wang, C. G. Prosko, G. Badawy, S. Gazibegovic, Y. Liu, P. Krogstrup, E. P. Bakkers, *et al.*, arXiv preprint arXiv:2110.03257 (2021).
[5] G. Burkard, D. Loss, and D. P. DiVincenzo, Physical Review B **59**, 2070 (1999).
[6] D. Stepanenko, N. E. Bonesteel, D. P. DiVincenzo, G. Burkard, and D. Loss, Physical Review B **68**, 115306 (2003).
[7] S. Nadj-Perge, V. Pribiag, J. Van den Berg, K. Zuo, S. Plissard, E. Bakkers, S. Frolov, and L. Kouwenhoven, Physical review letters **108**, 166801 (2012).
[8] T. Duty, G. Johansson, K. Bladh, D. Gunnarsson, C. Wilson, and P. Delsing, Physical review letters **95**, 206807 (2005).
[9] K. Petersson, C. Smith, D. Anderson, P. Atkinson, G. Jones, and D. Ritchie, Nano letters **10**, 2789 (2010).
[10] M. Urdampilleta, A. Chatterjee, C. C. Lo, T. Kobayashi, J. Mansir, S. Barraud, A. C. Betz, S. Rogge, M. F. Gonzalez-Zalba, and J. J. Morton, Physical Review X **5**, 031024 (2015).
[11] R. Mizuta, R. Otxoa, A. Betz, and M. F. Gonzalez-Zalba, Physical Review B **95**, 045414 (2017).
[12] Z. Scherübl, A. Pályi, G. Frank, I. E. Lukács, G. Fülöp, B. Fülöp, J. Nygård, K. Watanabe, T. Taniguchi, G. Zaránd, *et al.*, Communications Physics **2**, 1 (2019).
